# Supplementary material for: Improved estimate of the cross section for inverse beta decay
Source: arXiv:1601.06169 ancillary file (2016-01-22)
Supplement: Supplementary file 1 [file SupplementalMaterial.pdf]

# Improved estimate of the cross section for inverse beta decay. Supplemental Material


Artur M. Ankowski*

*Center for Neutrino Physics, Virginia Tech, Blacksburg, Virginia 24061, USA*


To facilitate implementation of the results of this article, an example of a C++ program for the differential cross section $d\sigma_{\rm cvc}/d\cos\theta$ is provided in `program.zip`. This Supplemental Material presents CVC corrections to the formula of Vogel and Beacom [1] and to the next-to-leading order approximation of the cross section derived by Strumia and Vissani [2]. Finally, off-the-mass-shell expressions in the de Forest approximation are also presented.

In Table I, the IBD cross section of this article is compared with the estimates in the approaches of Strumia and Vissani [2], Vogel and Beacom [1], and Llewellyn-Smith [3]. The energy is expressed in MeV, and the cross sections are given in units of $10^{-42}$ cm$^2$, with $a$e-00$x$ denoting $a\times10^{-x}$. Additionally, numerical results for energies up to 500 MeV are given in the files `TCS_CC_anue_p_1026_SV.txt` [2], `TCS_CC_anue_p_VB.txt` [1], and `TCS_CC_anue_p_1026_LS.txt` [3].

## APPROXIMATED EXPRESSIONS

Following Vogel and Beacom [1], $\sigma^{\rm tree}_{\rm cvc}$ may be expanded in powers of $1/M$, keeping terms up to next to leading order. The result reads

$$\left(\frac{d\sigma}{d\cos\theta}\right)^{(1)}=\frac{\sigma_0}{2}\left\{(f^2+3g^2)+(f^2-g^2)v_e^{(1)}\cos\theta+zf^2\frac{m_e^2}{q^2_{(1)}}\frac{\Delta}{E_\nu E_e^{(1)}}\left[E_\nu+E_e^{(1)}+\left(1+\frac{m_e^2}{q^2_{(1)}}\right)\frac{\Delta}{2}\right]\right\}E_e^{(1)}p_e^{(1)} -\frac{\sigma_0}{2}\frac{\Gamma}{M}E_e^{(0)}p_e^{(0)},\tag{1}$$

where $q^2_{(i)}=m_e^2-2E_\nu E_e^{(i)}(1-v_e^{(i)}\cos\theta)$ and

$$\begin{aligned}\Gamma=&\,2(f+f_2)g\left[(2E_e^{(0)}+\Delta)(1-v_e^{(0)}\cos\theta)-\frac{m_e^2}{E_e^{(0)}}\right]+(f^2+g^2)\left[\Delta(1+v_e^{(0)}\cos\theta)+\frac{m_e^2}{E_e^{(0)}}\right]\\&+\left[(f^2+3g^2)+(f^2-g^2)v_e^{(0)}\cos\theta\right]\left[(E_e^{(0)}+\Delta)\left(1-\frac{\cos\theta}{v_e^{(0)}}\right)-\Delta\right]\\&+zf^2\frac{m_e^2}{q^2_{(0)}}\frac{\Delta}{2}\left[\left(4+\frac{3\Delta}{E_e^{(0)}}+\frac{\Delta}{E_e^{(0)}}\frac{m_e^2}{q^2_{(0)}}\right)\left(1-\frac{\cos\theta}{v_e^{(0)}}\right)+\frac{m_e^2}{E_\nu E_e^{(0)}}\left(1-\frac{\Delta^2}{q^2_{(0)}}\right)-\frac{2\Delta}{E_e^{(0)}}\right].\end{aligned}\tag{2}$$

In the above equations, the notation and sign conventions of Ref. [1] are applied.

On the other hand, an approximated formula valid to higher energies has been proposed by Strumia and Vissani [2]. Including the CVC-related terms, it can be cast in the form

$$\frac{d\sigma^{\rm tree}_{\rm NLO}}{d\cos\theta}=\mathcal{J}\frac{(G_F\cos\theta_C)^2}{8\pi M_p^2E_\nu^2}\left[M^4A+M^2B(s-u)+C(s-u)^2\right],\tag{3}$$

with higher-order terms neglected only in the coefficients

$$\begin{aligned}A&=4(\tau+\mu)\left(F_A^2-F_1^2\right)-8\mu\frac{\Delta}{M}\left(F_1+F_2\right)F_A-\frac{\Delta^2}{M^2}\left(F_1^2+F_A^2\right)-z\frac{\Delta^2}{M^2}\frac{\mu}{\tau}\left(1-\frac{\mu}{\tau}\right)F_1^2,\\B&=4\tau\left(F_1+F_2\right)F_A-z\frac{\Delta}{M}\frac{\mu}{\tau}F_1^2,\\C&=\frac{1}{4}\left(F_1^2+F_A^2\right),\end{aligned}\tag{4}$$

and the Jacobian $\mathcal{J}$ equal to

$$\mathcal{J}=\frac{dq^2}{d\cos\theta}=\frac{2M_pE_\nu|\mathbf{k}'|^2}{CE_e-B|\mathbf{k}'|}\tag{5}$$

where $|\mathbf{k}'| = \sqrt{E_e^2 - m^2}$, $E_e = E_\nu - \omega$, and

$$\omega = \frac{A^2 B - E_\nu C^2 - C\sqrt{(A^2 - BE_\nu)^2 - m^2(B^2 - C^2)}}{B^2 - C^2} \tag{6}$$

with

$$\begin{aligned} A^2 &= E_\nu^2 + M\Delta - m^2/2, \\ B &= M_p + E_\nu, \\ C &= E_\nu \cos\theta. \end{aligned} \tag{7}$$

## OFF-THE-MASS-SHELL EXPRESSIONS

When neutrino scatters on a bound nucleon, the on-shell expression for the contraction of the leptonic and hadronic tensors, $L_{\mu\nu}$ and $\widetilde{H}^{\mu\nu}$, is no longer valid. The appropriate formula reads then

$$L_{\mu\nu}\widetilde{H}^{\mu\nu} = 2\sum_{j=1}^{5} A_j \widetilde{H}_j, \tag{8}$$

where the kinematic coefficients $A_j$ are equal to

$$\begin{aligned} A_1 &= 2M^2 k\cdot k', \\ A_2 &= 2\widetilde{p}\cdot k\, \widetilde{p}\cdot k' - M^2 k\cdot k', \\ A_3 &= 2(\widetilde{p}\cdot k'\, k\cdot\widetilde{q} - \widetilde{p}\cdot k\, k'\cdot\widetilde{q}), \\ A_4 &= 2k\cdot\widetilde{q}\, k'\cdot\widetilde{q} - k\cdot k'\, \widetilde{q}^2, \\ A_5 &= 2(\widetilde{p}\cdot k\, k'\cdot\widetilde{q} + \widetilde{p}\cdot k'\, k\cdot\widetilde{q} - k\cdot k'\, \widetilde{p}\cdot\widetilde{q}), \end{aligned} \tag{9}$$

with $\widetilde{p} = (E_N, \mathbf{p})$ denoting the initial nucleon's four-momentum and $\widetilde{q} = (E'_N - E_N, \mathbf{p}' - \mathbf{p})$ being the four-momentum transferred to the nucleon. The structure functions $\widetilde{H}_j$ are related to the nucleon form factors by

$$\begin{aligned} \widetilde{H}_1 &= \left(\tau + \frac{\Delta^2}{4M^2}\right)(F_1+F_2)^2 + (1+\tau)F_A^2, \\ \widetilde{H}_2 &= F_1^2 + \tau F_2^2 + F_A^2, \\ \widetilde{H}_3 &= (F_1+F_2)F_A, \\ \widetilde{H}_4 &= \left(\tau + \frac{\Delta^2}{4M^2}\right)F_P^2 - \left(1 - \frac{\Delta}{2M}\right)F_P F_A + \frac{1}{4}\left(F_1^2 + \tau F_2^2\right) - \frac{1}{4}(F_1+F_2)^2 + \frac{\Delta}{4M}F_2^2 \\ &\quad + \frac{z}{\tau}\frac{\Delta}{4M}F_1^2\left[1 + \left(\frac{1}{\tau} - 1\right)\frac{\Delta}{4M}\right] + \frac{\Delta}{4M}F_1F_2\left[1 - z - \frac{z}{\tau}\frac{\Delta}{2M}\right], \\ \widetilde{H}_5 &= \frac{1}{2}H_2 + \frac{\Delta}{4M}\left[\frac{z}{\tau}F_1^2 + (1-z)F_1F_2 + F_2^2 + 2F_PF_A\right], \end{aligned} \tag{10}$$

with $\tau = -\widetilde{q}^2/(4M^2)$. In the case of neutrino scattering, the signs of $\widetilde{H}_3$ and $\Delta$ are reversed.

TABLE I: Estimates of the IBD cross section.

| $E_\nu$ | CVC | Strumia–Vissani | Vogel–Beacom | Llewellyn-Smith |
|---|---|---|---|---|
| 1.80 | 0.000e+000 | 0.000e+000 | 0.000e+000 | 2.969e-001 |
| 1.81 | 2.814e-003 | 3.169e-003 | 3.164e-003 | 3.004e-001 |
| 1.82 | 5.442e-003 | 6.107e-003 | 6.104e-003 | 3.038e-001 |
| 1.83 | 7.327e-003 | 8.193e-003 | 8.190e-003 | 3.073e-001 |
| 1.84 | 8.956e-003 | 9.982e-003 | 9.980e-003 | 3.107e-001 |
| 1.85 | 1.046e-002 | 1.162e-002 | 1.162e-002 | 3.142e-001 |
| 1.86 | 1.188e-002 | 1.316e-002 | 1.316e-002 | 3.178e-001 |
| 1.87 | 1.326e-002 | 1.465e-002 | 1.465e-002 | 3.213e-001 |
| 1.88 | 1.461e-002 | 1.610e-002 | 1.609e-002 | 3.248e-001 |
| 1.89 | 1.595e-002 | 1.752e-002 | 1.752e-002 | 3.284e-001 |
| 1.90 | 1.727e-002 | 1.892e-002 | 1.892e-002 | 3.320e-001 |

| | | | | |
|---|---|---|---|---|
| 1.91 | 1.859e-002 | 2.032e-002 | 2.032e-002 | 3.356e-001 |
| 1.92 | 1.991e-002 | 2.171e-002 | 2.171e-002 | 3.392e-001 |
| 1.93 | 2.124e-002 | 2.310e-002 | 2.310e-002 | 3.429e-001 |
| 1.94 | 2.256e-002 | 2.450e-002 | 2.449e-002 | 3.465e-001 |
| 1.95 | 2.390e-002 | 2.589e-002 | 2.589e-002 | 3.502e-001 |
| 1.96 | 2.525e-002 | 2.730e-002 | 2.729e-002 | 3.539e-001 |
| 1.97 | 2.661e-002 | 2.871e-002 | 2.871e-002 | 3.576e-001 |
| 1.98 | 2.797e-002 | 3.013e-002 | 3.013e-002 | 3.614e-001 |
| 1.99 | 2.936e-002 | 3.156e-002 | 3.156e-002 | 3.651e-001 |
| 2.00 | 3.075e-002 | 3.300e-002 | 3.300e-002 | 3.689e-001 |
| 2.01 | 3.216e-002 | 3.446e-002 | 3.446e-002 | 3.727e-001 |
| 2.02 | 3.358e-002 | 3.593e-002 | 3.592e-002 | 3.765e-001 |
| 2.03 | 3.502e-002 | 3.741e-002 | 3.740e-002 | 3.803e-001 |
| 2.04 | 3.648e-002 | 3.890e-002 | 3.890e-002 | 3.842e-001 |
| 2.05 | 3.795e-002 | 4.041e-002 | 4.041e-002 | 3.880e-001 |
| 2.06 | 3.943e-002 | 4.193e-002 | 4.193e-002 | 3.919e-001 |
| 2.07 | 4.093e-002 | 4.347e-002 | 4.347e-002 | 3.958e-001 |
| 2.08 | 4.245e-002 | 4.503e-002 | 4.502e-002 | 3.997e-001 |
| 2.09 | 4.399e-002 | 4.660e-002 | 4.659e-002 | 4.037e-001 |
| 2.10 | 4.554e-002 | 4.818e-002 | 4.818e-002 | 4.076e-001 |
| 2.11 | 4.711e-002 | 4.978e-002 | 4.978e-002 | 4.116e-001 |
| 2.12 | 4.870e-002 | 5.140e-002 | 5.139e-002 | 4.156e-001 |
| 2.13 | 5.030e-002 | 5.303e-002 | 5.303e-002 | 4.196e-001 |
| 2.14 | 5.192e-002 | 5.468e-002 | 5.468e-002 | 4.237e-001 |
| 2.15 | 5.356e-002 | 5.635e-002 | 5.635e-002 | 4.277e-001 |
| 2.16 | 5.522e-002 | 5.804e-002 | 5.803e-002 | 4.318e-001 |
| 2.17 | 5.690e-002 | 5.974e-002 | 5.973e-002 | 4.358e-001 |
| 2.18 | 5.859e-002 | 6.145e-002 | 6.145e-002 | 4.400e-001 |
| 2.19 | 6.030e-002 | 6.319e-002 | 6.318e-002 | 4.441e-001 |
| 2.20 | 6.203e-002 | 6.494e-002 | 6.494e-002 | 4.482e-001 |
| 2.21 | 6.378e-002 | 6.671e-002 | 6.671e-002 | 4.524e-001 |
| 2.22 | 6.554e-002 | 6.850e-002 | 6.849e-002 | 4.565e-001 |
| 2.23 | 6.733e-002 | 7.031e-002 | 7.030e-002 | 4.607e-001 |
| 2.24 | 6.913e-002 | 7.213e-002 | 7.212e-002 | 4.650e-001 |
| 2.25 | 7.095e-002 | 7.397e-002 | 7.396e-002 | 4.692e-001 |
| 2.26 | 7.279e-002 | 7.583e-002 | 7.582e-002 | 4.734e-001 |
| 2.27 | 7.464e-002 | 7.770e-002 | 7.769e-002 | 4.777e-001 |
| 2.28 | 7.652e-002 | 7.960e-002 | 7.959e-002 | 4.820e-001 |
| 2.29 | 7.841e-002 | 8.151e-002 | 8.150e-002 | 4.863e-001 |
| 2.30 | 8.032e-002 | 8.344e-002 | 8.343e-002 | 4.906e-001 |
| 2.31 | 8.225e-002 | 8.538e-002 | 8.538e-002 | 4.950e-001 |
| 2.32 | 8.420e-002 | 8.735e-002 | 8.734e-002 | 4.993e-001 |
| 2.33 | 8.617e-002 | 8.933e-002 | 8.932e-002 | 5.037e-001 |
| 2.34 | 8.815e-002 | 9.134e-002 | 9.132e-002 | 5.081e-001 |
| 2.35 | 9.016e-002 | 9.335e-002 | 9.334e-002 | 5.125e-001 |
| 2.36 | 9.218e-002 | 9.539e-002 | 9.538e-002 | 5.169e-001 |
| 2.37 | 9.422e-002 | 9.745e-002 | 9.744e-002 | 5.214e-001 |
| 2.38 | 9.628e-002 | 9.952e-002 | 9.951e-002 | 5.258e-001 |
| 2.39 | 9.836e-002 | 1.016e-001 | 1.016e-001 | 5.303e-001 |
| 2.40 | 1.005e-001 | 1.037e-001 | 1.037e-001 | 5.348e-001 |
| 2.41 | 1.026e-001 | 1.059e-001 | 1.058e-001 | 5.394e-001 |
| 2.42 | 1.047e-001 | 1.080e-001 | 1.080e-001 | 5.439e-001 |
| 2.43 | 1.069e-001 | 1.102e-001 | 1.101e-001 | 5.484e-001 |
| 2.44 | 1.090e-001 | 1.123e-001 | 1.123e-001 | 5.530e-001 |
| 2.45 | 1.112e-001 | 1.145e-001 | 1.145e-001 | 5.576e-001 |
| 2.46 | 1.134e-001 | 1.168e-001 | 1.168e-001 | 5.622e-001 |
| 2.47 | 1.157e-001 | 1.190e-001 | 1.190e-001 | 5.669e-001 |
| 2.48 | 1.179e-001 | 1.213e-001 | 1.212e-001 | 5.715e-001 |
| 2.49 | 1.202e-001 | 1.235e-001 | 1.235e-001 | 5.762e-001 |
| 2.50 | 1.224e-001 | 1.258e-001 | 1.258e-001 | 5.809e-001 |
| 2.51 | 1.247e-001 | 1.281e-001 | 1.281e-001 | 5.856e-001 |
| 2.52 | 1.271e-001 | 1.305e-001 | 1.305e-001 | 5.903e-001 |
| 2.53 | 1.294e-001 | 1.328e-001 | 1.328e-001 | 5.950e-001 |
| 2.54 | 1.318e-001 | 1.352e-001 | 1.352e-001 | 5.998e-001 |
| 2.55 | 1.341e-001 | 1.376e-001 | 1.375e-001 | 6.046e-001 |
| 2.56 | 1.365e-001 | 1.400e-001 | 1.399e-001 | 6.094e-001 |
| 2.57 | 1.389e-001 | 1.424e-001 | 1.424e-001 | 6.142e-001 |
| 2.58 | 1.414e-001 | 1.448e-001 | 1.448e-001 | 6.190e-001 |
| 2.59 | 1.438e-001 | 1.473e-001 | 1.473e-001 | 6.239e-001 |
| 2.60 | 1.463e-001 | 1.498e-001 | 1.497e-001 | 6.287e-001 |
| 2.61 | 1.488e-001 | 1.523e-001 | 1.522e-001 | 6.336e-001 |
| 2.62 | 1.513e-001 | 1.548e-001 | 1.547e-001 | 6.385e-001 |
| 2.63 | 1.538e-001 | 1.573e-001 | 1.573e-001 | 6.434e-001 |
| 2.64 | 1.564e-001 | 1.599e-001 | 1.598e-001 | 6.484e-001 |
| 2.65 | 1.589e-001 | 1.624e-001 | 1.624e-001 | 6.533e-001 |
| 2.66 | 1.615e-001 | 1.650e-001 | 1.650e-001 | 6.583e-001 |
| 2.67 | 1.641e-001 | 1.676e-001 | 1.676e-001 | 6.633e-001 |
| 2.68 | 1.667e-001 | 1.702e-001 | 1.702e-001 | 6.683e-001 |
| 2.69 | 1.693e-001 | 1.729e-001 | 1.728e-001 | 6.733e-001 |
| 2.70 | 1.720e-001 | 1.755e-001 | 1.755e-001 | 6.784e-001 |
| 2.71 | 1.747e-001 | 1.782e-001 | 1.782e-001 | 6.835e-001 |
| 2.72 | 1.774e-001 | 1.809e-001 | 1.809e-001 | 6.885e-001 |
| 2.73 | 1.801e-001 | 1.836e-001 | 1.836e-001 | 6.936e-001 |

| | | | | |
|---|---|---|---|---|
| 2.74 | 1.828e-001 | 1.864e-001 | 1.863e-001 | 6.988e-001 |
| 2.75 | 1.855e-001 | 1.891e-001 | 1.891e-001 | 7.039e-001 |
| 2.76 | 1.883e-001 | 1.919e-001 | 1.918e-001 | 7.091e-001 |
| 2.77 | 1.911e-001 | 1.947e-001 | 1.946e-001 | 7.142e-001 |
| 2.78 | 1.939e-001 | 1.975e-001 | 1.974e-001 | 7.194e-001 |
| 2.79 | 1.967e-001 | 2.003e-001 | 2.003e-001 | 7.246e-001 |
| 2.80 | 1.996e-001 | 2.031e-001 | 2.031e-001 | 7.299e-001 |
| 2.81 | 2.024e-001 | 2.060e-001 | 2.060e-001 | 7.351e-001 |
| 2.82 | 2.053e-001 | 2.089e-001 | 2.089e-001 | 7.404e-001 |
| 2.83 | 2.082e-001 | 2.118e-001 | 2.117e-001 | 7.456e-001 |
| 2.84 | 2.111e-001 | 2.147e-001 | 2.147e-001 | 7.509e-001 |
| 2.85 | 2.140e-001 | 2.176e-001 | 2.176e-001 | 7.563e-001 |
| 2.86 | 2.170e-001 | 2.206e-001 | 2.206e-001 | 7.616e-001 |
| 2.87 | 2.200e-001 | 2.236e-001 | 2.235e-001 | 7.670e-001 |
| 2.88 | 2.229e-001 | 2.266e-001 | 2.265e-001 | 7.723e-001 |
| 2.89 | 2.259e-001 | 2.296e-001 | 2.295e-001 | 7.777e-001 |
| 2.90 | 2.290e-001 | 2.326e-001 | 2.325e-001 | 7.831e-001 |
| 2.91 | 2.320e-001 | 2.356e-001 | 2.356e-001 | 7.886e-001 |
| 2.92 | 2.351e-001 | 2.387e-001 | 2.387e-001 | 7.940e-001 |
| 2.93 | 2.382e-001 | 2.418e-001 | 2.417e-001 | 7.995e-001 |
| 2.94 | 2.412e-001 | 2.449e-001 | 2.448e-001 | 8.049e-001 |
| 2.95 | 2.444e-001 | 2.480e-001 | 2.480e-001 | 8.104e-001 |
| 2.96 | 2.475e-001 | 2.511e-001 | 2.511e-001 | 8.160e-001 |
| 2.97 | 2.507e-001 | 2.543e-001 | 2.542e-001 | 8.215e-001 |
| 2.98 | 2.538e-001 | 2.575e-001 | 2.574e-001 | 8.270e-001 |
| 2.99 | 2.570e-001 | 2.607e-001 | 2.606e-001 | 8.326e-001 |
| 3.00 | 2.602e-001 | 2.639e-001 | 2.638e-001 | 8.382e-001 |
| 3.01 | 2.635e-001 | 2.671e-001 | 2.671e-001 | 8.438e-001 |
| 3.02 | 2.667e-001 | 2.704e-001 | 2.703e-001 | 8.494e-001 |
| 3.03 | 2.700e-001 | 2.736e-001 | 2.736e-001 | 8.551e-001 |
| 3.04 | 2.732e-001 | 2.769e-001 | 2.768e-001 | 8.607e-001 |
| 3.05 | 2.765e-001 | 2.802e-001 | 2.801e-001 | 8.664e-001 |
| 3.06 | 2.799e-001 | 2.835e-001 | 2.835e-001 | 8.721e-001 |
| 3.07 | 2.832e-001 | 2.869e-001 | 2.868e-001 | 8.778e-001 |
| 3.08 | 2.866e-001 | 2.902e-001 | 2.902e-001 | 8.835e-001 |
| 3.09 | 2.899e-001 | 2.936e-001 | 2.935e-001 | 8.893e-001 |
| 3.10 | 2.933e-001 | 2.970e-001 | 2.969e-001 | 8.951e-001 |
| 3.11 | 2.967e-001 | 3.004e-001 | 3.003e-001 | 9.008e-001 |
| 3.12 | 3.002e-001 | 3.038e-001 | 3.038e-001 | 9.066e-001 |
| 3.13 | 3.036e-001 | 3.073e-001 | 3.072e-001 | 9.125e-001 |
| 3.14 | 3.071e-001 | 3.108e-001 | 3.107e-001 | 9.183e-001 |
| 3.15 | 3.106e-001 | 3.142e-001 | 3.142e-001 | 9.242e-001 |
| 3.16 | 3.141e-001 | 3.177e-001 | 3.177e-001 | 9.300e-001 |
| 3.17 | 3.176e-001 | 3.213e-001 | 3.212e-001 | 9.359e-001 |
| 3.18 | 3.211e-001 | 3.248e-001 | 3.247e-001 | 9.418e-001 |
| 3.19 | 3.247e-001 | 3.284e-001 | 3.283e-001 | 9.478e-001 |
| 3.20 | 3.283e-001 | 3.319e-001 | 3.319e-001 | 9.537e-001 |
| 3.21 | 3.319e-001 | 3.355e-001 | 3.355e-001 | 9.597e-001 |
| 3.22 | 3.355e-001 | 3.392e-001 | 3.391e-001 | 9.657e-001 |
| 3.23 | 3.391e-001 | 3.428e-001 | 3.427e-001 | 9.717e-001 |
| 3.24 | 3.428e-001 | 3.464e-001 | 3.464e-001 | 9.777e-001 |
| 3.25 | 3.464e-001 | 3.501e-001 | 3.500e-001 | 9.837e-001 |
| 3.26 | 3.501e-001 | 3.538e-001 | 3.537e-001 | 9.898e-001 |
| 3.27 | 3.538e-001 | 3.575e-001 | 3.574e-001 | 9.958e-001 |
| 3.28 | 3.575e-001 | 3.612e-001 | 3.611e-001 | 1.002e+000 |
| 3.29 | 3.613e-001 | 3.650e-001 | 3.649e-001 | 1.008e+000 |
| 3.30 | 3.650e-001 | 3.687e-001 | 3.686e-001 | 1.014e+000 |
| 3.31 | 3.688e-001 | 3.725e-001 | 3.724e-001 | 1.020e+000 |
| 3.32 | 3.726e-001 | 3.763e-001 | 3.762e-001 | 1.026e+000 |
| 3.33 | 3.764e-001 | 3.801e-001 | 3.800e-001 | 1.033e+000 |
| 3.34 | 3.803e-001 | 3.839e-001 | 3.838e-001 | 1.039e+000 |
| 3.35 | 3.841e-001 | 3.878e-001 | 3.877e-001 | 1.045e+000 |
| 3.36 | 3.880e-001 | 3.917e-001 | 3.916e-001 | 1.051e+000 |
| 3.37 | 3.919e-001 | 3.955e-001 | 3.954e-001 | 1.058e+000 |
| 3.38 | 3.958e-001 | 3.995e-001 | 3.993e-001 | 1.064e+000 |
| 3.39 | 3.997e-001 | 4.034e-001 | 4.033e-001 | 1.070e+000 |
| 3.40 | 4.036e-001 | 4.073e-001 | 4.072e-001 | 1.076e+000 |
| 3.41 | 4.076e-001 | 4.113e-001 | 4.112e-001 | 1.083e+000 |
| 3.42 | 4.116e-001 | 4.153e-001 | 4.151e-001 | 1.089e+000 |
| 3.43 | 4.156e-001 | 4.193e-001 | 4.191e-001 | 1.095e+000 |
| 3.44 | 4.196e-001 | 4.233e-001 | 4.232e-001 | 1.102e+000 |
| 3.45 | 4.236e-001 | 4.273e-001 | 4.272e-001 | 1.108e+000 |
| 3.46 | 4.277e-001 | 4.314e-001 | 4.312e-001 | 1.115e+000 |
| 3.47 | 4.317e-001 | 4.354e-001 | 4.353e-001 | 1.121e+000 |
| 3.48 | 4.358e-001 | 4.395e-001 | 4.394e-001 | 1.127e+000 |
| 3.49 | 4.399e-001 | 4.436e-001 | 4.435e-001 | 1.134e+000 |
| 3.50 | 4.441e-001 | 4.477e-001 | 4.476e-001 | 1.140e+000 |
| 3.51 | 4.482e-001 | 4.519e-001 | 4.518e-001 | 1.147e+000 |
| 3.52 | 4.524e-001 | 4.560e-001 | 4.559e-001 | 1.153e+000 |
| 3.53 | 4.566e-001 | 4.602e-001 | 4.601e-001 | 1.160e+000 |
| 3.54 | 4.607e-001 | 4.644e-001 | 4.643e-001 | 1.166e+000 |
| 3.55 | 4.650e-001 | 4.686e-001 | 4.685e-001 | 1.173e+000 |
| 3.56 | 4.692e-001 | 4.729e-001 | 4.727e-001 | 1.180e+000 |

| | | | | |
|---|---|---|---|---|
| 3.57 | 4.734e-001 | 4.771e-001 | 4.770e-001 | 1.186e+000 |
| 3.58 | 4.777e-001 | 4.814e-001 | 4.812e-001 | 1.193e+000 |
| 3.59 | 4.820e-001 | 4.857e-001 | 4.855e-001 | 1.199e+000 |
| 3.60 | 4.863e-001 | 4.900e-001 | 4.898e-001 | 1.206e+000 |
| 3.61 | 4.906e-001 | 4.943e-001 | 4.941e-001 | 1.213e+000 |
| 3.62 | 4.950e-001 | 4.986e-001 | 4.985e-001 | 1.219e+000 |
| 3.63 | 4.993e-001 | 5.030e-001 | 5.028e-001 | 1.226e+000 |
| 3.64 | 5.037e-001 | 5.074e-001 | 5.072e-001 | 1.233e+000 |
| 3.65 | 5.081e-001 | 5.118e-001 | 5.116e-001 | 1.240e+000 |
| 3.66 | 5.125e-001 | 5.162e-001 | 5.160e-001 | 1.246e+000 |
| 3.67 | 5.170e-001 | 5.206e-001 | 5.205e-001 | 1.253e+000 |
| 3.68 | 5.214e-001 | 5.251e-001 | 5.249e-001 | 1.260e+000 |
| 3.69 | 5.259e-001 | 5.295e-001 | 5.294e-001 | 1.267e+000 |
| 3.70 | 5.304e-001 | 5.340e-001 | 5.338e-001 | 1.274e+000 |
| 3.71 | 5.349e-001 | 5.385e-001 | 5.384e-001 | 1.280e+000 |
| 3.72 | 5.394e-001 | 5.430e-001 | 5.429e-001 | 1.287e+000 |
| 3.73 | 5.439e-001 | 5.476e-001 | 5.474e-001 | 1.294e+000 |
| 3.74 | 5.485e-001 | 5.521e-001 | 5.520e-001 | 1.301e+000 |
| 3.75 | 5.531e-001 | 5.567e-001 | 5.565e-001 | 1.308e+000 |
| 3.76 | 5.577e-001 | 5.613e-001 | 5.611e-001 | 1.315e+000 |
| 3.77 | 5.623e-001 | 5.659e-001 | 5.657e-001 | 1.322e+000 |
| 3.78 | 5.669e-001 | 5.706e-001 | 5.704e-001 | 1.329e+000 |
| 3.79 | 5.716e-001 | 5.752e-001 | 5.750e-001 | 1.336e+000 |
| 3.80 | 5.762e-001 | 5.799e-001 | 5.797e-001 | 1.343e+000 |
| 3.81 | 5.809e-001 | 5.846e-001 | 5.844e-001 | 1.350e+000 |
| 3.82 | 5.856e-001 | 5.893e-001 | 5.891e-001 | 1.357e+000 |
| 3.83 | 5.904e-001 | 5.940e-001 | 5.938e-001 | 1.364e+000 |
| 3.84 | 5.951e-001 | 5.987e-001 | 5.985e-001 | 1.371e+000 |
| 3.85 | 5.999e-001 | 6.035e-001 | 6.033e-001 | 1.378e+000 |
| 3.86 | 6.046e-001 | 6.083e-001 | 6.080e-001 | 1.385e+000 |
| 3.87 | 6.094e-001 | 6.130e-001 | 6.128e-001 | 1.392e+000 |
| 3.88 | 6.142e-001 | 6.179e-001 | 6.176e-001 | 1.400e+000 |
| 3.89 | 6.191e-001 | 6.227e-001 | 6.225e-001 | 1.407e+000 |
| 3.90 | 6.239e-001 | 6.275e-001 | 6.273e-001 | 1.414e+000 |
| 3.91 | 6.288e-001 | 6.324e-001 | 6.322e-001 | 1.421e+000 |
| 3.92 | 6.337e-001 | 6.373e-001 | 6.370e-001 | 1.428e+000 |
| 3.93 | 6.386e-001 | 6.422e-001 | 6.419e-001 | 1.436e+000 |
| 3.94 | 6.435e-001 | 6.471e-001 | 6.469e-001 | 1.443e+000 |
| 3.95 | 6.484e-001 | 6.520e-001 | 6.518e-001 | 1.450e+000 |
| 3.96 | 6.534e-001 | 6.570e-001 | 6.567e-001 | 1.457e+000 |
| 3.97 | 6.584e-001 | 6.620e-001 | 6.617e-001 | 1.465e+000 |
| 3.98 | 6.633e-001 | 6.670e-001 | 6.667e-001 | 1.472e+000 |
| 3.99 | 6.684e-001 | 6.720e-001 | 6.717e-001 | 1.479e+000 |
| 4.00 | 6.734e-001 | 6.770e-001 | 6.767e-001 | 1.487e+000 |
| 4.01 | 6.784e-001 | 6.820e-001 | 6.818e-001 | 1.494e+000 |
| 4.02 | 6.835e-001 | 6.871e-001 | 6.868e-001 | 1.502e+000 |
| 4.03 | 6.886e-001 | 6.922e-001 | 6.919e-001 | 1.509e+000 |
| 4.04 | 6.937e-001 | 6.973e-001 | 6.970e-001 | 1.516e+000 |
| 4.05 | 6.988e-001 | 7.024e-001 | 7.021e-001 | 1.524e+000 |
| 4.06 | 7.039e-001 | 7.075e-001 | 7.072e-001 | 1.531e+000 |
| 4.07 | 7.091e-001 | 7.127e-001 | 7.124e-001 | 1.539e+000 |
| 4.08 | 7.143e-001 | 7.178e-001 | 7.176e-001 | 1.546e+000 |
| 4.09 | 7.194e-001 | 7.230e-001 | 7.227e-001 | 1.554e+000 |
| 4.10 | 7.247e-001 | 7.282e-001 | 7.279e-001 | 1.561e+000 |
| 4.11 | 7.299e-001 | 7.335e-001 | 7.332e-001 | 1.569e+000 |
| 4.12 | 7.351e-001 | 7.387e-001 | 7.384e-001 | 1.576e+000 |
| 4.13 | 7.404e-001 | 7.440e-001 | 7.437e-001 | 1.584e+000 |
| 4.14 | 7.457e-001 | 7.492e-001 | 7.489e-001 | 1.592e+000 |
| 4.15 | 7.510e-001 | 7.545e-001 | 7.542e-001 | 1.599e+000 |
| 4.16 | 7.563e-001 | 7.598e-001 | 7.595e-001 | 1.607e+000 |
| 4.17 | 7.616e-001 | 7.652e-001 | 7.649e-001 | 1.615e+000 |
| 4.18 | 7.670e-001 | 7.705e-001 | 7.702e-001 | 1.622e+000 |
| 4.19 | 7.723e-001 | 7.759e-001 | 7.756e-001 | 1.630e+000 |
| 4.20 | 7.777e-001 | 7.813e-001 | 7.809e-001 | 1.638e+000 |
| 4.21 | 7.831e-001 | 7.867e-001 | 7.863e-001 | 1.645e+000 |
| 4.22 | 7.885e-001 | 7.921e-001 | 7.918e-001 | 1.653e+000 |
| 4.23 | 7.940e-001 | 7.975e-001 | 7.972e-001 | 1.661e+000 |
| 4.24 | 7.994e-001 | 8.030e-001 | 8.026e-001 | 1.669e+000 |
| 4.25 | 8.049e-001 | 8.085e-001 | 8.081e-001 | 1.676e+000 |
| 4.26 | 8.104e-001 | 8.140e-001 | 8.136e-001 | 1.684e+000 |
| 4.27 | 8.159e-001 | 8.195e-001 | 8.191e-001 | 1.692e+000 |
| 4.28 | 8.215e-001 | 8.250e-001 | 8.246e-001 | 1.700e+000 |
| 4.29 | 8.270e-001 | 8.305e-001 | 8.302e-001 | 1.708e+000 |
| 4.30 | 8.326e-001 | 8.361e-001 | 8.357e-001 | 1.716e+000 |
| 4.31 | 8.381e-001 | 8.417e-001 | 8.413e-001 | 1.724e+000 |
| 4.32 | 8.438e-001 | 8.473e-001 | 8.469e-001 | 1.732e+000 |
| 4.33 | 8.494e-001 | 8.529e-001 | 8.525e-001 | 1.739e+000 |
| 4.34 | 8.550e-001 | 8.585e-001 | 8.581e-001 | 1.747e+000 |
| 4.35 | 8.607e-001 | 8.642e-001 | 8.638e-001 | 1.755e+000 |
| 4.36 | 8.663e-001 | 8.699e-001 | 8.695e-001 | 1.763e+000 |
| 4.37 | 8.720e-001 | 8.755e-001 | 8.751e-001 | 1.771e+000 |
| 4.38 | 8.777e-001 | 8.812e-001 | 8.808e-001 | 1.779e+000 |
| 4.39 | 8.835e-001 | 8.870e-001 | 8.866e-001 | 1.787e+000 |

| | | | | |
|---|---|---|---|---|
| 4.40 | 8.892e-001 | 8.927e-001 | 8.923e-001 | 1.795e+000 |
| 4.41 | 8.950e-001 | 8.985e-001 | 8.980e-001 | 1.804e+000 |
| 4.42 | 9.007e-001 | 9.042e-001 | 9.038e-001 | 1.812e+000 |
| 4.43 | 9.065e-001 | 9.100e-001 | 9.096e-001 | 1.820e+000 |
| 4.44 | 9.123e-001 | 9.159e-001 | 9.154e-001 | 1.828e+000 |
| 4.45 | 9.182e-001 | 9.217e-001 | 9.212e-001 | 1.836e+000 |
| 4.46 | 9.240e-001 | 9.275e-001 | 9.271e-001 | 1.844e+000 |
| 4.47 | 9.299e-001 | 9.334e-001 | 9.329e-001 | 1.852e+000 |
| 4.48 | 9.358e-001 | 9.393e-001 | 9.388e-001 | 1.861e+000 |
| 4.49 | 9.417e-001 | 9.452e-001 | 9.447e-001 | 1.869e+000 |
| 4.50 | 9.476e-001 | 9.511e-001 | 9.506e-001 | 1.877e+000 |
| 4.51 | 9.535e-001 | 9.570e-001 | 9.566e-001 | 1.885e+000 |
| 4.52 | 9.595e-001 | 9.630e-001 | 9.625e-001 | 1.894e+000 |
| 4.53 | 9.655e-001 | 9.690e-001 | 9.685e-001 | 1.902e+000 |
| 4.54 | 9.715e-001 | 9.750e-001 | 9.745e-001 | 1.910e+000 |
| 4.55 | 9.775e-001 | 9.810e-001 | 9.805e-001 | 1.918e+000 |
| 4.56 | 9.835e-001 | 9.870e-001 | 9.865e-001 | 1.927e+000 |
| 4.57 | 9.895e-001 | 9.930e-001 | 9.925e-001 | 1.935e+000 |
| 4.58 | 9.956e-001 | 9.991e-001 | 9.986e-001 | 1.943e+000 |
| 4.59 | 1.002e+000 | 1.005e+000 | 1.005e+000 | 1.952e+000 |
| 4.60 | 1.008e+000 | 1.011e+000 | 1.011e+000 | 1.960e+000 |
| 4.61 | 1.014e+000 | 1.017e+000 | 1.017e+000 | 1.969e+000 |
| 4.62 | 1.020e+000 | 1.023e+000 | 1.023e+000 | 1.977e+000 |
| 4.63 | 1.026e+000 | 1.030e+000 | 1.029e+000 | 1.986e+000 |
| 4.64 | 1.032e+000 | 1.036e+000 | 1.035e+000 | 1.994e+000 |
| 4.65 | 1.039e+000 | 1.042e+000 | 1.041e+000 | 2.003e+000 |
| 4.66 | 1.045e+000 | 1.048e+000 | 1.048e+000 | 2.011e+000 |
| 4.67 | 1.051e+000 | 1.054e+000 | 1.054e+000 | 2.020e+000 |
| 4.68 | 1.057e+000 | 1.061e+000 | 1.060e+000 | 2.028e+000 |
| 4.69 | 1.063e+000 | 1.067e+000 | 1.066e+000 | 2.037e+000 |
| 4.70 | 1.070e+000 | 1.073e+000 | 1.073e+000 | 2.045e+000 |
| 4.71 | 1.076e+000 | 1.079e+000 | 1.079e+000 | 2.054e+000 |
| 4.72 | 1.082e+000 | 1.086e+000 | 1.085e+000 | 2.062e+000 |
| 4.73 | 1.089e+000 | 1.092e+000 | 1.092e+000 | 2.071e+000 |
| 4.74 | 1.095e+000 | 1.098e+000 | 1.098e+000 | 2.080e+000 |
| 4.75 | 1.101e+000 | 1.105e+000 | 1.104e+000 | 2.088e+000 |
| 4.76 | 1.108e+000 | 1.111e+000 | 1.111e+000 | 2.097e+000 |
| 4.77 | 1.114e+000 | 1.118e+000 | 1.117e+000 | 2.106e+000 |
| 4.78 | 1.121e+000 | 1.124e+000 | 1.123e+000 | 2.114e+000 |
| 4.79 | 1.127e+000 | 1.130e+000 | 1.130e+000 | 2.123e+000 |
| 4.80 | 1.133e+000 | 1.137e+000 | 1.136e+000 | 2.132e+000 |
| 4.81 | 1.140e+000 | 1.143e+000 | 1.143e+000 | 2.141e+000 |
| 4.82 | 1.146e+000 | 1.150e+000 | 1.149e+000 | 2.149e+000 |
| 4.83 | 1.153e+000 | 1.156e+000 | 1.156e+000 | 2.158e+000 |
| 4.84 | 1.159e+000 | 1.163e+000 | 1.162e+000 | 2.167e+000 |
| 4.85 | 1.166e+000 | 1.169e+000 | 1.169e+000 | 2.176e+000 |
| 4.86 | 1.173e+000 | 1.176e+000 | 1.175e+000 | 2.185e+000 |
| 4.87 | 1.179e+000 | 1.183e+000 | 1.182e+000 | 2.194e+000 |
| 4.88 | 1.186e+000 | 1.189e+000 | 1.188e+000 | 2.202e+000 |
| 4.89 | 1.192e+000 | 1.196e+000 | 1.195e+000 | 2.211e+000 |
| 4.90 | 1.199e+000 | 1.202e+000 | 1.202e+000 | 2.220e+000 |
| 4.91 | 1.206e+000 | 1.209e+000 | 1.208e+000 | 2.229e+000 |
| 4.92 | 1.212e+000 | 1.216e+000 | 1.215e+000 | 2.238e+000 |
| 4.93 | 1.219e+000 | 1.222e+000 | 1.222e+000 | 2.247e+000 |
| 4.94 | 1.226e+000 | 1.229e+000 | 1.228e+000 | 2.256e+000 |
| 4.95 | 1.232e+000 | 1.236e+000 | 1.235e+000 | 2.265e+000 |
| 4.96 | 1.239e+000 | 1.242e+000 | 1.242e+000 | 2.274e+000 |
| 4.97 | 1.246e+000 | 1.249e+000 | 1.248e+000 | 2.283e+000 |
| 4.98 | 1.253e+000 | 1.256e+000 | 1.255e+000 | 2.292e+000 |
| 4.99 | 1.259e+000 | 1.263e+000 | 1.262e+000 | 2.301e+000 |
| 5.00 | 1.266e+000 | 1.270e+000 | 1.269e+000 | 2.310e+000 |
| 5.01 | 1.273e+000 | 1.276e+000 | 1.276e+000 | 2.320e+000 |
| 5.02 | 1.280e+000 | 1.283e+000 | 1.282e+000 | 2.329e+000 |
| 5.03 | 1.287e+000 | 1.290e+000 | 1.289e+000 | 2.338e+000 |
| 5.04 | 1.294e+000 | 1.297e+000 | 1.296e+000 | 2.347e+000 |
| 5.05 | 1.300e+000 | 1.304e+000 | 1.303e+000 | 2.356e+000 |
| 5.06 | 1.307e+000 | 1.311e+000 | 1.310e+000 | 2.365e+000 |
| 5.07 | 1.314e+000 | 1.318e+000 | 1.317e+000 | 2.375e+000 |
| 5.08 | 1.321e+000 | 1.325e+000 | 1.324e+000 | 2.384e+000 |
| 5.09 | 1.328e+000 | 1.332e+000 | 1.331e+000 | 2.393e+000 |
| 5.10 | 1.335e+000 | 1.339e+000 | 1.338e+000 | 2.402e+000 |
| 5.11 | 1.342e+000 | 1.345e+000 | 1.345e+000 | 2.412e+000 |
| 5.12 | 1.349e+000 | 1.353e+000 | 1.352e+000 | 2.421e+000 |
| 5.13 | 1.356e+000 | 1.360e+000 | 1.359e+000 | 2.430e+000 |
| 5.14 | 1.363e+000 | 1.367e+000 | 1.366e+000 | 2.439e+000 |
| 5.15 | 1.370e+000 | 1.374e+000 | 1.373e+000 | 2.449e+000 |
| 5.16 | 1.377e+000 | 1.381e+000 | 1.380e+000 | 2.458e+000 |
| 5.17 | 1.384e+000 | 1.388e+000 | 1.387e+000 | 2.468e+000 |
| 5.18 | 1.392e+000 | 1.395e+000 | 1.394e+000 | 2.477e+000 |
| 5.19 | 1.399e+000 | 1.402e+000 | 1.401e+000 | 2.486e+000 |
| 5.20 | 1.406e+000 | 1.409e+000 | 1.408e+000 | 2.496e+000 |
| 5.21 | 1.413e+000 | 1.416e+000 | 1.415e+000 | 2.505e+000 |
| 5.22 | 1.420e+000 | 1.424e+000 | 1.423e+000 | 2.515e+000 |

| | | | | |
|---|---|---|---|---|
| 5.23 | 1.427e+000 | 1.431e+000 | 1.430e+000 | 2.524e+000 |
| 5.24 | 1.435e+000 | 1.438e+000 | 1.437e+000 | 2.534e+000 |
| 5.25 | 1.442e+000 | 1.445e+000 | 1.444e+000 | 2.543e+000 |
| 5.26 | 1.449e+000 | 1.452e+000 | 1.451e+000 | 2.553e+000 |
| 5.27 | 1.456e+000 | 1.460e+000 | 1.459e+000 | 2.562e+000 |
| 5.28 | 1.464e+000 | 1.467e+000 | 1.466e+000 | 2.572e+000 |
| 5.29 | 1.471e+000 | 1.474e+000 | 1.473e+000 | 2.581e+000 |
| 5.30 | 1.478e+000 | 1.482e+000 | 1.481e+000 | 2.591e+000 |
| 5.31 | 1.486e+000 | 1.489e+000 | 1.488e+000 | 2.601e+000 |
| 5.32 | 1.493e+000 | 1.496e+000 | 1.495e+000 | 2.610e+000 |
| 5.33 | 1.500e+000 | 1.504e+000 | 1.503e+000 | 2.620e+000 |
| 5.34 | 1.508e+000 | 1.511e+000 | 1.510e+000 | 2.630e+000 |
| 5.35 | 1.515e+000 | 1.519e+000 | 1.517e+000 | 2.639e+000 |
| 5.36 | 1.523e+000 | 1.526e+000 | 1.525e+000 | 2.649e+000 |
| 5.37 | 1.530e+000 | 1.533e+000 | 1.532e+000 | 2.659e+000 |
| 5.38 | 1.538e+000 | 1.541e+000 | 1.540e+000 | 2.668e+000 |
| 5.39 | 1.545e+000 | 1.548e+000 | 1.547e+000 | 2.678e+000 |
| 5.40 | 1.553e+000 | 1.556e+000 | 1.555e+000 | 2.688e+000 |
| 5.41 | 1.560e+000 | 1.563e+000 | 1.562e+000 | 2.698e+000 |
| 5.42 | 1.568e+000 | 1.571e+000 | 1.570e+000 | 2.708e+000 |
| 5.43 | 1.575e+000 | 1.578e+000 | 1.577e+000 | 2.717e+000 |
| 5.44 | 1.583e+000 | 1.586e+000 | 1.585e+000 | 2.727e+000 |
| 5.45 | 1.590e+000 | 1.594e+000 | 1.592e+000 | 2.737e+000 |
| 5.46 | 1.598e+000 | 1.601e+000 | 1.600e+000 | 2.747e+000 |
| 5.47 | 1.606e+000 | 1.609e+000 | 1.608e+000 | 2.757e+000 |
| 5.48 | 1.613e+000 | 1.616e+000 | 1.615e+000 | 2.767e+000 |
| 5.49 | 1.621e+000 | 1.624e+000 | 1.623e+000 | 2.777e+000 |
| 5.50 | 1.629e+000 | 1.632e+000 | 1.631e+000 | 2.787e+000 |
| 5.51 | 1.636e+000 | 1.639e+000 | 1.638e+000 | 2.796e+000 |
| 5.52 | 1.644e+000 | 1.647e+000 | 1.646e+000 | 2.806e+000 |
| 5.53 | 1.652e+000 | 1.655e+000 | 1.654e+000 | 2.816e+000 |
| 5.54 | 1.659e+000 | 1.663e+000 | 1.661e+000 | 2.826e+000 |
| 5.55 | 1.667e+000 | 1.670e+000 | 1.669e+000 | 2.836e+000 |
| 5.56 | 1.675e+000 | 1.678e+000 | 1.677e+000 | 2.847e+000 |
| 5.57 | 1.683e+000 | 1.686e+000 | 1.685e+000 | 2.857e+000 |
| 5.58 | 1.691e+000 | 1.694e+000 | 1.692e+000 | 2.867e+000 |
| 5.59 | 1.698e+000 | 1.702e+000 | 1.700e+000 | 2.877e+000 |
| 5.60 | 1.706e+000 | 1.709e+000 | 1.708e+000 | 2.887e+000 |
| 5.61 | 1.714e+000 | 1.717e+000 | 1.716e+000 | 2.897e+000 |
| 5.62 | 1.722e+000 | 1.725e+000 | 1.724e+000 | 2.907e+000 |
| 5.63 | 1.730e+000 | 1.733e+000 | 1.732e+000 | 2.917e+000 |
| 5.64 | 1.738e+000 | 1.741e+000 | 1.740e+000 | 2.927e+000 |
| 5.65 | 1.746e+000 | 1.749e+000 | 1.747e+000 | 2.938e+000 |
| 5.66 | 1.754e+000 | 1.757e+000 | 1.755e+000 | 2.948e+000 |
| 5.67 | 1.762e+000 | 1.765e+000 | 1.763e+000 | 2.958e+000 |
| 5.68 | 1.770e+000 | 1.773e+000 | 1.771e+000 | 2.968e+000 |
| 5.69 | 1.778e+000 | 1.781e+000 | 1.779e+000 | 2.979e+000 |
| 5.70 | 1.786e+000 | 1.789e+000 | 1.787e+000 | 2.989e+000 |
| 5.71 | 1.794e+000 | 1.797e+000 | 1.795e+000 | 2.999e+000 |
| 5.72 | 1.802e+000 | 1.805e+000 | 1.803e+000 | 3.009e+000 |
| 5.73 | 1.810e+000 | 1.813e+000 | 1.811e+000 | 3.020e+000 |
| 5.74 | 1.818e+000 | 1.821e+000 | 1.820e+000 | 3.030e+000 |
| 5.75 | 1.826e+000 | 1.829e+000 | 1.828e+000 | 3.040e+000 |
| 5.76 | 1.834e+000 | 1.837e+000 | 1.836e+000 | 3.051e+000 |
| 5.77 | 1.842e+000 | 1.845e+000 | 1.844e+000 | 3.061e+000 |
| 5.78 | 1.850e+000 | 1.854e+000 | 1.852e+000 | 3.072e+000 |
| 5.79 | 1.859e+000 | 1.862e+000 | 1.860e+000 | 3.082e+000 |
| 5.80 | 1.867e+000 | 1.870e+000 | 1.868e+000 | 3.092e+000 |
| 5.81 | 1.875e+000 | 1.878e+000 | 1.876e+000 | 3.103e+000 |
| 5.82 | 1.883e+000 | 1.886e+000 | 1.885e+000 | 3.113e+000 |
| 5.83 | 1.891e+000 | 1.895e+000 | 1.893e+000 | 3.124e+000 |
| 5.84 | 1.900e+000 | 1.903e+000 | 1.901e+000 | 3.134e+000 |
| 5.85 | 1.908e+000 | 1.911e+000 | 1.909e+000 | 3.145e+000 |
| 5.86 | 1.916e+000 | 1.919e+000 | 1.918e+000 | 3.155e+000 |
| 5.87 | 1.925e+000 | 1.928e+000 | 1.926e+000 | 3.166e+000 |
| 5.88 | 1.933e+000 | 1.936e+000 | 1.934e+000 | 3.177e+000 |
| 5.89 | 1.941e+000 | 1.944e+000 | 1.943e+000 | 3.187e+000 |
| 5.90 | 1.950e+000 | 1.953e+000 | 1.951e+000 | 3.198e+000 |
| 5.91 | 1.958e+000 | 1.961e+000 | 1.959e+000 | 3.208e+000 |
| 5.92 | 1.966e+000 | 1.969e+000 | 1.968e+000 | 3.219e+000 |
| 5.93 | 1.975e+000 | 1.978e+000 | 1.976e+000 | 3.230e+000 |
| 5.94 | 1.983e+000 | 1.986e+000 | 1.985e+000 | 3.240e+000 |
| 5.95 | 1.992e+000 | 1.995e+000 | 1.993e+000 | 3.251e+000 |
| 5.96 | 2.000e+000 | 2.003e+000 | 2.001e+000 | 3.262e+000 |
| 5.97 | 2.009e+000 | 2.012e+000 | 2.010e+000 | 3.273e+000 |
| 5.98 | 2.017e+000 | 2.020e+000 | 2.018e+000 | 3.283e+000 |
| 5.99 | 2.026e+000 | 2.029e+000 | 2.027e+000 | 3.294e+000 |
| 6.00 | 2.034e+000 | 2.037e+000 | 2.035e+000 | 3.305e+000 |
| 6.01 | 2.043e+000 | 2.046e+000 | 2.044e+000 | 3.316e+000 |
| 6.02 | 2.051e+000 | 2.054e+000 | 2.052e+000 | 3.326e+000 |
| 6.03 | 2.060e+000 | 2.063e+000 | 2.061e+000 | 3.337e+000 |
| 6.04 | 2.068e+000 | 2.072e+000 | 2.070e+000 | 3.348e+000 |
| 6.05 | 2.077e+000 | 2.080e+000 | 2.078e+000 | 3.359e+000 |

| | | | | |
|---|---|---|---|---|
| 6.06 | 2.086e+000 | 2.089e+000 | 2.087e+000 | 3.370e+000 |
| 6.07 | 2.094e+000 | 2.097e+000 | 2.095e+000 | 3.381e+000 |
| 6.08 | 2.103e+000 | 2.106e+000 | 2.104e+000 | 3.392e+000 |
| 6.09 | 2.112e+000 | 2.115e+000 | 2.113e+000 | 3.403e+000 |
| 6.10 | 2.120e+000 | 2.124e+000 | 2.121e+000 | 3.413e+000 |
| 6.11 | 2.129e+000 | 2.132e+000 | 2.130e+000 | 3.424e+000 |
| 6.12 | 2.138e+000 | 2.141e+000 | 2.139e+000 | 3.435e+000 |
| 6.13 | 2.147e+000 | 2.150e+000 | 2.148e+000 | 3.446e+000 |
| 6.14 | 2.155e+000 | 2.158e+000 | 2.156e+000 | 3.457e+000 |
| 6.15 | 2.164e+000 | 2.167e+000 | 2.165e+000 | 3.468e+000 |
| 6.16 | 2.173e+000 | 2.176e+000 | 2.174e+000 | 3.479e+000 |
| 6.17 | 2.182e+000 | 2.185e+000 | 2.183e+000 | 3.491e+000 |
| 6.18 | 2.191e+000 | 2.194e+000 | 2.192e+000 | 3.502e+000 |
| 6.19 | 2.200e+000 | 2.203e+000 | 2.200e+000 | 3.513e+000 |
| 6.20 | 2.208e+000 | 2.211e+000 | 2.209e+000 | 3.524e+000 |
| 6.21 | 2.217e+000 | 2.220e+000 | 2.218e+000 | 3.535e+000 |
| 6.22 | 2.226e+000 | 2.229e+000 | 2.227e+000 | 3.546e+000 |
| 6.23 | 2.235e+000 | 2.238e+000 | 2.236e+000 | 3.557e+000 |
| 6.24 | 2.244e+000 | 2.247e+000 | 2.245e+000 | 3.568e+000 |
| 6.25 | 2.253e+000 | 2.256e+000 | 2.254e+000 | 3.580e+000 |
| 6.26 | 2.262e+000 | 2.265e+000 | 2.263e+000 | 3.591e+000 |
| 6.27 | 2.271e+000 | 2.274e+000 | 2.272e+000 | 3.602e+000 |
| 6.28 | 2.280e+000 | 2.283e+000 | 2.281e+000 | 3.613e+000 |
| 6.29 | 2.289e+000 | 2.292e+000 | 2.290e+000 | 3.625e+000 |
| 6.30 | 2.298e+000 | 2.301e+000 | 2.299e+000 | 3.636e+000 |
| 6.31 | 2.307e+000 | 2.310e+000 | 2.308e+000 | 3.647e+000 |
| 6.32 | 2.316e+000 | 2.319e+000 | 2.317e+000 | 3.658e+000 |
| 6.33 | 2.325e+000 | 2.328e+000 | 2.326e+000 | 3.670e+000 |
| 6.34 | 2.334e+000 | 2.337e+000 | 2.335e+000 | 3.681e+000 |
| 6.35 | 2.344e+000 | 2.347e+000 | 2.344e+000 | 3.692e+000 |
| 6.36 | 2.353e+000 | 2.356e+000 | 2.353e+000 | 3.704e+000 |
| 6.37 | 2.362e+000 | 2.365e+000 | 2.362e+000 | 3.715e+000 |
| 6.38 | 2.371e+000 | 2.374e+000 | 2.372e+000 | 3.727e+000 |
| 6.39 | 2.380e+000 | 2.383e+000 | 2.381e+000 | 3.738e+000 |
| 6.40 | 2.389e+000 | 2.392e+000 | 2.390e+000 | 3.749e+000 |
| 6.41 | 2.399e+000 | 2.402e+000 | 2.399e+000 | 3.761e+000 |
| 6.42 | 2.408e+000 | 2.411e+000 | 2.408e+000 | 3.772e+000 |
| 6.43 | 2.417e+000 | 2.420e+000 | 2.418e+000 | 3.784e+000 |
| 6.44 | 2.426e+000 | 2.429e+000 | 2.427e+000 | 3.795e+000 |
| 6.45 | 2.436e+000 | 2.439e+000 | 2.436e+000 | 3.807e+000 |
| 6.46 | 2.445e+000 | 2.448e+000 | 2.445e+000 | 3.818e+000 |
| 6.47 | 2.454e+000 | 2.457e+000 | 2.455e+000 | 3.830e+000 |
| 6.48 | 2.464e+000 | 2.467e+000 | 2.464e+000 | 3.842e+000 |
| 6.49 | 2.473e+000 | 2.476e+000 | 2.473e+000 | 3.853e+000 |
| 6.50 | 2.482e+000 | 2.486e+000 | 2.483e+000 | 3.865e+000 |
| 6.51 | 2.492e+000 | 2.495e+000 | 2.492e+000 | 3.876e+000 |
| 6.52 | 2.501e+000 | 2.504e+000 | 2.502e+000 | 3.888e+000 |
| 6.53 | 2.511e+000 | 2.514e+000 | 2.511e+000 | 3.900e+000 |
| 6.54 | 2.520e+000 | 2.523e+000 | 2.520e+000 | 3.911e+000 |
| 6.55 | 2.530e+000 | 2.533e+000 | 2.530e+000 | 3.923e+000 |
| 6.56 | 2.539e+000 | 2.542e+000 | 2.539e+000 | 3.935e+000 |
| 6.57 | 2.549e+000 | 2.552e+000 | 2.549e+000 | 3.946e+000 |
| 6.58 | 2.558e+000 | 2.561e+000 | 2.558e+000 | 3.958e+000 |
| 6.59 | 2.568e+000 | 2.571e+000 | 2.568e+000 | 3.970e+000 |
| 6.60 | 2.577e+000 | 2.580e+000 | 2.577e+000 | 3.982e+000 |
| 6.61 | 2.587e+000 | 2.590e+000 | 2.587e+000 | 3.993e+000 |
| 6.62 | 2.596e+000 | 2.599e+000 | 2.596e+000 | 4.005e+000 |
| 6.63 | 2.606e+000 | 2.609e+000 | 2.606e+000 | 4.017e+000 |
| 6.64 | 2.616e+000 | 2.619e+000 | 2.616e+000 | 4.029e+000 |
| 6.65 | 2.625e+000 | 2.628e+000 | 2.625e+000 | 4.041e+000 |
| 6.66 | 2.635e+000 | 2.638e+000 | 2.635e+000 | 4.053e+000 |
| 6.67 | 2.645e+000 | 2.648e+000 | 2.644e+000 | 4.065e+000 |
| 6.68 | 2.654e+000 | 2.657e+000 | 2.654e+000 | 4.076e+000 |
| 6.69 | 2.664e+000 | 2.667e+000 | 2.664e+000 | 4.088e+000 |
| 6.70 | 2.674e+000 | 2.677e+000 | 2.673e+000 | 4.100e+000 |
| 6.71 | 2.683e+000 | 2.686e+000 | 2.683e+000 | 4.112e+000 |
| 6.72 | 2.693e+000 | 2.696e+000 | 2.693e+000 | 4.124e+000 |
| 6.73 | 2.703e+000 | 2.706e+000 | 2.703e+000 | 4.136e+000 |
| 6.74 | 2.713e+000 | 2.716e+000 | 2.712e+000 | 4.148e+000 |
| 6.75 | 2.723e+000 | 2.725e+000 | 2.722e+000 | 4.160e+000 |
| 6.76 | 2.732e+000 | 2.735e+000 | 2.732e+000 | 4.172e+000 |
| 6.77 | 2.742e+000 | 2.745e+000 | 2.742e+000 | 4.184e+000 |
| 6.78 | 2.752e+000 | 2.755e+000 | 2.752e+000 | 4.196e+000 |
| 6.79 | 2.762e+000 | 2.765e+000 | 2.761e+000 | 4.208e+000 |
| 6.80 | 2.772e+000 | 2.775e+000 | 2.771e+000 | 4.220e+000 |
| 6.81 | 2.782e+000 | 2.785e+000 | 2.781e+000 | 4.233e+000 |
| 6.82 | 2.792e+000 | 2.795e+000 | 2.791e+000 | 4.245e+000 |
| 6.83 | 2.802e+000 | 2.804e+000 | 2.801e+000 | 4.257e+000 |
| 6.84 | 2.811e+000 | 2.814e+000 | 2.811e+000 | 4.269e+000 |
| 6.85 | 2.821e+000 | 2.824e+000 | 2.821e+000 | 4.281e+000 |
| 6.86 | 2.831e+000 | 2.834e+000 | 2.831e+000 | 4.293e+000 |
| 6.87 | 2.841e+000 | 2.844e+000 | 2.841e+000 | 4.306e+000 |
| 6.88 | 2.851e+000 | 2.854e+000 | 2.851e+000 | 4.318e+000 |

| | | | | |
|---|---|---|---|---|
| 6.89 | 2.862e+000 | 2.864e+000 | 2.861e+000 | 4.330e+000 |
| 6.90 | 2.872e+000 | 2.875e+000 | 2.871e+000 | 4.342e+000 |
| 6.91 | 2.882e+000 | 2.885e+000 | 2.881e+000 | 4.355e+000 |
| 6.92 | 2.892e+000 | 2.895e+000 | 2.891e+000 | 4.367e+000 |
| 6.93 | 2.902e+000 | 2.905e+000 | 2.901e+000 | 4.379e+000 |
| 6.94 | 2.912e+000 | 2.915e+000 | 2.911e+000 | 4.392e+000 |
| 6.95 | 2.922e+000 | 2.925e+000 | 2.921e+000 | 4.404e+000 |
| 6.96 | 2.932e+000 | 2.935e+000 | 2.931e+000 | 4.416e+000 |
| 6.97 | 2.942e+000 | 2.945e+000 | 2.942e+000 | 4.429e+000 |
| 6.98 | 2.953e+000 | 2.956e+000 | 2.952e+000 | 4.441e+000 |
| 6.99 | 2.963e+000 | 2.966e+000 | 2.962e+000 | 4.453e+000 |
| 7.00 | 2.973e+000 | 2.976e+000 | 2.972e+000 | 4.466e+000 |
| 7.01 | 2.983e+000 | 2.986e+000 | 2.982e+000 | 4.478e+000 |
| 7.02 | 2.994e+000 | 2.996e+000 | 2.993e+000 | 4.491e+000 |
| 7.03 | 3.004e+000 | 3.007e+000 | 3.003e+000 | 4.503e+000 |
| 7.04 | 3.014e+000 | 3.017e+000 | 3.013e+000 | 4.516e+000 |
| 7.05 | 3.024e+000 | 3.027e+000 | 3.023e+000 | 4.528e+000 |
| 7.06 | 3.035e+000 | 3.038e+000 | 3.034e+000 | 4.541e+000 |
| 7.07 | 3.045e+000 | 3.048e+000 | 3.044e+000 | 4.553e+000 |
| 7.08 | 3.055e+000 | 3.058e+000 | 3.054e+000 | 4.566e+000 |
| 7.09 | 3.066e+000 | 3.069e+000 | 3.065e+000 | 4.578e+000 |
| 7.10 | 3.076e+000 | 3.079e+000 | 3.075e+000 | 4.591e+000 |
| 7.11 | 3.087e+000 | 3.089e+000 | 3.085e+000 | 4.604e+000 |
| 7.12 | 3.097e+000 | 3.100e+000 | 3.096e+000 | 4.616e+000 |
| 7.13 | 3.107e+000 | 3.110e+000 | 3.106e+000 | 4.629e+000 |
| 7.14 | 3.118e+000 | 3.121e+000 | 3.117e+000 | 4.641e+000 |
| 7.15 | 3.128e+000 | 3.131e+000 | 3.127e+000 | 4.654e+000 |
| 7.16 | 3.139e+000 | 3.142e+000 | 3.137e+000 | 4.667e+000 |
| 7.17 | 3.149e+000 | 3.152e+000 | 3.148e+000 | 4.679e+000 |
| 7.18 | 3.160e+000 | 3.163e+000 | 3.158e+000 | 4.692e+000 |
| 7.19 | 3.170e+000 | 3.173e+000 | 3.169e+000 | 4.705e+000 |
| 7.20 | 3.181e+000 | 3.184e+000 | 3.179e+000 | 4.718e+000 |
| 7.21 | 3.192e+000 | 3.194e+000 | 3.190e+000 | 4.730e+000 |
| 7.22 | 3.202e+000 | 3.205e+000 | 3.201e+000 | 4.743e+000 |
| 7.23 | 3.213e+000 | 3.216e+000 | 3.211e+000 | 4.756e+000 |
| 7.24 | 3.223e+000 | 3.226e+000 | 3.222e+000 | 4.769e+000 |
| 7.25 | 3.234e+000 | 3.237e+000 | 3.232e+000 | 4.782e+000 |
| 7.26 | 3.245e+000 | 3.247e+000 | 3.243e+000 | 4.795e+000 |
| 7.27 | 3.255e+000 | 3.258e+000 | 3.254e+000 | 4.807e+000 |
| 7.28 | 3.266e+000 | 3.269e+000 | 3.264e+000 | 4.820e+000 |
| 7.29 | 3.277e+000 | 3.280e+000 | 3.275e+000 | 4.833e+000 |
| 7.30 | 3.287e+000 | 3.290e+000 | 3.286e+000 | 4.846e+000 |
| 7.31 | 3.298e+000 | 3.301e+000 | 3.296e+000 | 4.859e+000 |
| 7.32 | 3.309e+000 | 3.312e+000 | 3.307e+000 | 4.872e+000 |
| 7.33 | 3.320e+000 | 3.323e+000 | 3.318e+000 | 4.885e+000 |
| 7.34 | 3.330e+000 | 3.333e+000 | 3.329e+000 | 4.898e+000 |
| 7.35 | 3.341e+000 | 3.344e+000 | 3.339e+000 | 4.911e+000 |
| 7.36 | 3.352e+000 | 3.355e+000 | 3.350e+000 | 4.924e+000 |
| 7.37 | 3.363e+000 | 3.366e+000 | 3.361e+000 | 4.937e+000 |
| 7.38 | 3.374e+000 | 3.377e+000 | 3.372e+000 | 4.950e+000 |
| 7.39 | 3.385e+000 | 3.387e+000 | 3.383e+000 | 4.963e+000 |
| 7.40 | 3.396e+000 | 3.398e+000 | 3.393e+000 | 4.976e+000 |
| 7.41 | 3.406e+000 | 3.409e+000 | 3.404e+000 | 4.989e+000 |
| 7.42 | 3.417e+000 | 3.420e+000 | 3.415e+000 | 5.002e+000 |
| 7.43 | 3.428e+000 | 3.431e+000 | 3.426e+000 | 5.015e+000 |
| 7.44 | 3.439e+000 | 3.442e+000 | 3.437e+000 | 5.028e+000 |
| 7.45 | 3.450e+000 | 3.453e+000 | 3.448e+000 | 5.042e+000 |
| 7.46 | 3.461e+000 | 3.464e+000 | 3.459e+000 | 5.055e+000 |
| 7.47 | 3.472e+000 | 3.475e+000 | 3.470e+000 | 5.068e+000 |
| 7.48 | 3.483e+000 | 3.486e+000 | 3.481e+000 | 5.081e+000 |
| 7.49 | 3.494e+000 | 3.497e+000 | 3.492e+000 | 5.094e+000 |
| 7.50 | 3.505e+000 | 3.508e+000 | 3.503e+000 | 5.108e+000 |
| 7.51 | 3.516e+000 | 3.519e+000 | 3.514e+000 | 5.121e+000 |
| 7.52 | 3.527e+000 | 3.530e+000 | 3.525e+000 | 5.134e+000 |
| 7.53 | 3.539e+000 | 3.541e+000 | 3.536e+000 | 5.147e+000 |
| 7.54 | 3.550e+000 | 3.552e+000 | 3.547e+000 | 5.161e+000 |
| 7.55 | 3.561e+000 | 3.564e+000 | 3.558e+000 | 5.174e+000 |
| 7.56 | 3.572e+000 | 3.575e+000 | 3.569e+000 | 5.187e+000 |
| 7.57 | 3.583e+000 | 3.586e+000 | 3.580e+000 | 5.201e+000 |
| 7.58 | 3.594e+000 | 3.597e+000 | 3.592e+000 | 5.214e+000 |
| 7.59 | 3.605e+000 | 3.608e+000 | 3.603e+000 | 5.227e+000 |
| 7.60 | 3.617e+000 | 3.619e+000 | 3.614e+000 | 5.241e+000 |
| 7.61 | 3.628e+000 | 3.631e+000 | 3.625e+000 | 5.254e+000 |
| 7.62 | 3.639e+000 | 3.642e+000 | 3.636e+000 | 5.268e+000 |
| 7.63 | 3.650e+000 | 3.653e+000 | 3.648e+000 | 5.281e+000 |
| 7.64 | 3.662e+000 | 3.664e+000 | 3.659e+000 | 5.294e+000 |
| 7.65 | 3.673e+000 | 3.676e+000 | 3.670e+000 | 5.308e+000 |
| 7.66 | 3.684e+000 | 3.687e+000 | 3.681e+000 | 5.321e+000 |
| 7.67 | 3.696e+000 | 3.698e+000 | 3.693e+000 | 5.335e+000 |
| 7.68 | 3.707e+000 | 3.710e+000 | 3.704e+000 | 5.348e+000 |
| 7.69 | 3.718e+000 | 3.721e+000 | 3.715e+000 | 5.362e+000 |
| 7.70 | 3.730e+000 | 3.733e+000 | 3.727e+000 | 5.376e+000 |
| 7.71 | 3.741e+000 | 3.744e+000 | 3.738e+000 | 5.389e+000 |

| | | | | |
|---|---|---|---|---|
| 7.72 | 3.753e+000 | 3.755e+000 | 3.749e+000 | 5.403e+000 |
| 7.73 | 3.764e+000 | 3.767e+000 | 3.761e+000 | 5.416e+000 |
| 7.74 | 3.775e+000 | 3.778e+000 | 3.772e+000 | 5.430e+000 |
| 7.75 | 3.787e+000 | 3.790e+000 | 3.784e+000 | 5.444e+000 |
| 7.76 | 3.798e+000 | 3.801e+000 | 3.795e+000 | 5.457e+000 |
| 7.77 | 3.810e+000 | 3.813e+000 | 3.806e+000 | 5.471e+000 |
| 7.78 | 3.821e+000 | 3.824e+000 | 3.818e+000 | 5.485e+000 |
| 7.79 | 3.833e+000 | 3.836e+000 | 3.829e+000 | 5.498e+000 |
| 7.80 | 3.844e+000 | 3.847e+000 | 3.841e+000 | 5.512e+000 |
| 7.81 | 3.856e+000 | 3.859e+000 | 3.852e+000 | 5.526e+000 |
| 7.82 | 3.868e+000 | 3.870e+000 | 3.864e+000 | 5.539e+000 |
| 7.83 | 3.879e+000 | 3.882e+000 | 3.876e+000 | 5.553e+000 |
| 7.84 | 3.891e+000 | 3.893e+000 | 3.887e+000 | 5.567e+000 |
| 7.85 | 3.902e+000 | 3.905e+000 | 3.899e+000 | 5.581e+000 |
| 7.86 | 3.914e+000 | 3.917e+000 | 3.910e+000 | 5.595e+000 |
| 7.87 | 3.926e+000 | 3.928e+000 | 3.922e+000 | 5.608e+000 |
| 7.88 | 3.937e+000 | 3.940e+000 | 3.934e+000 | 5.622e+000 |
| 7.89 | 3.949e+000 | 3.952e+000 | 3.945e+000 | 5.636e+000 |
| 7.90 | 3.961e+000 | 3.963e+000 | 3.957e+000 | 5.650e+000 |
| 7.91 | 3.972e+000 | 3.975e+000 | 3.969e+000 | 5.664e+000 |
| 7.92 | 3.984e+000 | 3.987e+000 | 3.980e+000 | 5.678e+000 |
| 7.93 | 3.996e+000 | 3.999e+000 | 3.992e+000 | 5.692e+000 |
| 7.94 | 4.008e+000 | 4.010e+000 | 4.004e+000 | 5.706e+000 |
| 7.95 | 4.020e+000 | 4.022e+000 | 4.015e+000 | 5.719e+000 |
| 7.96 | 4.031e+000 | 4.034e+000 | 4.027e+000 | 5.733e+000 |
| 7.97 | 4.043e+000 | 4.046e+000 | 4.039e+000 | 5.747e+000 |
| 7.98 | 4.055e+000 | 4.058e+000 | 4.051e+000 | 5.761e+000 |
| 7.99 | 4.067e+000 | 4.070e+000 | 4.063e+000 | 5.775e+000 |
| 8.00 | 4.079e+000 | 4.081e+000 | 4.074e+000 | 5.789e+000 |
| 8.01 | 4.091e+000 | 4.093e+000 | 4.086e+000 | 5.803e+000 |
| 8.02 | 4.103e+000 | 4.105e+000 | 4.098e+000 | 5.818e+000 |
| 8.03 | 4.114e+000 | 4.117e+000 | 4.110e+000 | 5.832e+000 |
| 8.04 | 4.126e+000 | 4.129e+000 | 4.122e+000 | 5.846e+000 |
| 8.05 | 4.138e+000 | 4.141e+000 | 4.134e+000 | 5.860e+000 |
| 8.06 | 4.150e+000 | 4.153e+000 | 4.146e+000 | 5.874e+000 |
| 8.07 | 4.162e+000 | 4.165e+000 | 4.158e+000 | 5.888e+000 |
| 8.08 | 4.174e+000 | 4.177e+000 | 4.170e+000 | 5.902e+000 |
| 8.09 | 4.186e+000 | 4.189e+000 | 4.182e+000 | 5.916e+000 |
| 8.10 | 4.198e+000 | 4.201e+000 | 4.194e+000 | 5.931e+000 |
| 8.11 | 4.210e+000 | 4.213e+000 | 4.206e+000 | 5.945e+000 |
| 8.12 | 4.222e+000 | 4.225e+000 | 4.218e+000 | 5.959e+000 |
| 8.13 | 4.234e+000 | 4.237e+000 | 4.230e+000 | 5.973e+000 |
| 8.14 | 4.247e+000 | 4.249e+000 | 4.242e+000 | 5.987e+000 |
| 8.15 | 4.259e+000 | 4.261e+000 | 4.254e+000 | 6.002e+000 |
| 8.16 | 4.271e+000 | 4.274e+000 | 4.266e+000 | 6.016e+000 |
| 8.17 | 4.283e+000 | 4.286e+000 | 4.278e+000 | 6.030e+000 |
| 8.18 | 4.295e+000 | 4.298e+000 | 4.290e+000 | 6.045e+000 |
| 8.19 | 4.307e+000 | 4.310e+000 | 4.302e+000 | 6.059e+000 |
| 8.20 | 4.320e+000 | 4.322e+000 | 4.314e+000 | 6.073e+000 |
| 8.21 | 4.332e+000 | 4.334e+000 | 4.326e+000 | 6.088e+000 |
| 8.22 | 4.344e+000 | 4.347e+000 | 4.339e+000 | 6.102e+000 |
| 8.23 | 4.356e+000 | 4.359e+000 | 4.351e+000 | 6.116e+000 |
| 8.24 | 4.368e+000 | 4.371e+000 | 4.363e+000 | 6.131e+000 |
| 8.25 | 4.381e+000 | 4.383e+000 | 4.375e+000 | 6.145e+000 |
| 8.26 | 4.393e+000 | 4.396e+000 | 4.388e+000 | 6.160e+000 |
| 8.27 | 4.405e+000 | 4.408e+000 | 4.400e+000 | 6.174e+000 |
| 8.28 | 4.418e+000 | 4.420e+000 | 4.412e+000 | 6.189e+000 |
| 8.29 | 4.430e+000 | 4.433e+000 | 4.424e+000 | 6.203e+000 |
| 8.30 | 4.442e+000 | 4.445e+000 | 4.437e+000 | 6.218e+000 |
| 8.31 | 4.455e+000 | 4.457e+000 | 4.449e+000 | 6.232e+000 |
| 8.32 | 4.467e+000 | 4.470e+000 | 4.461e+000 | 6.247e+000 |
| 8.33 | 4.479e+000 | 4.482e+000 | 4.474e+000 | 6.261e+000 |
| 8.34 | 4.492e+000 | 4.495e+000 | 4.486e+000 | 6.276e+000 |
| 8.35 | 4.504e+000 | 4.507e+000 | 4.498e+000 | 6.290e+000 |
| 8.36 | 4.517e+000 | 4.519e+000 | 4.511e+000 | 6.305e+000 |
| 8.37 | 4.529e+000 | 4.532e+000 | 4.523e+000 | 6.320e+000 |
| 8.38 | 4.542e+000 | 4.544e+000 | 4.536e+000 | 6.334e+000 |
| 8.39 | 4.554e+000 | 4.557e+000 | 4.548e+000 | 6.349e+000 |
| 8.40 | 4.567e+000 | 4.569e+000 | 4.561e+000 | 6.364e+000 |
| 8.41 | 4.579e+000 | 4.582e+000 | 4.573e+000 | 6.378e+000 |
| 8.42 | 4.592e+000 | 4.594e+000 | 4.586e+000 | 6.393e+000 |
| 8.43 | 4.604e+000 | 4.607e+000 | 4.598e+000 | 6.408e+000 |
| 8.44 | 4.617e+000 | 4.620e+000 | 4.611e+000 | 6.422e+000 |
| 8.45 | 4.630e+000 | 4.632e+000 | 4.623e+000 | 6.437e+000 |
| 8.46 | 4.642e+000 | 4.645e+000 | 4.636e+000 | 6.452e+000 |
| 8.47 | 4.655e+000 | 4.657e+000 | 4.648e+000 | 6.467e+000 |
| 8.48 | 4.667e+000 | 4.670e+000 | 4.661e+000 | 6.481e+000 |
| 8.49 | 4.680e+000 | 4.683e+000 | 4.674e+000 | 6.496e+000 |
| 8.50 | 4.693e+000 | 4.695e+000 | 4.686e+000 | 6.511e+000 |
| 8.51 | 4.706e+000 | 4.708e+000 | 4.699e+000 | 6.526e+000 |
| 8.52 | 4.718e+000 | 4.721e+000 | 4.712e+000 | 6.541e+000 |
| 8.53 | 4.731e+000 | 4.734e+000 | 4.724e+000 | 6.555e+000 |
| 8.54 | 4.744e+000 | 4.746e+000 | 4.737e+000 | 6.570e+000 |

| | | | | |
|---|---|---|---|---|
| 8.55 | 4.756e+000 | 4.759e+000 | 4.750e+000 | 6.585e+000 |
| 8.56 | 4.769e+000 | 4.772e+000 | 4.762e+000 | 6.600e+000 |
| 8.57 | 4.782e+000 | 4.785e+000 | 4.775e+000 | 6.615e+000 |
| 8.58 | 4.795e+000 | 4.797e+000 | 4.788e+000 | 6.630e+000 |
| 8.59 | 4.808e+000 | 4.810e+000 | 4.801e+000 | 6.645e+000 |
| 8.60 | 4.820e+000 | 4.823e+000 | 4.813e+000 | 6.660e+000 |
| 8.61 | 4.833e+000 | 4.836e+000 | 4.826e+000 | 6.675e+000 |
| 8.62 | 4.846e+000 | 4.849e+000 | 4.839e+000 | 6.690e+000 |
| 8.63 | 4.859e+000 | 4.862e+000 | 4.852e+000 | 6.705e+000 |
| 8.64 | 4.872e+000 | 4.875e+000 | 4.865e+000 | 6.720e+000 |
| 8.65 | 4.885e+000 | 4.888e+000 | 4.878e+000 | 6.735e+000 |
| 8.66 | 4.898e+000 | 4.900e+000 | 4.890e+000 | 6.750e+000 |
| 8.67 | 4.911e+000 | 4.913e+000 | 4.903e+000 | 6.765e+000 |
| 8.68 | 4.924e+000 | 4.926e+000 | 4.916e+000 | 6.780e+000 |
| 8.69 | 4.937e+000 | 4.939e+000 | 4.929e+000 | 6.795e+000 |
| 8.70 | 4.950e+000 | 4.952e+000 | 4.942e+000 | 6.811e+000 |
| 8.71 | 4.963e+000 | 4.965e+000 | 4.955e+000 | 6.826e+000 |
| 8.72 | 4.976e+000 | 4.978e+000 | 4.968e+000 | 6.841e+000 |
| 8.73 | 4.989e+000 | 4.991e+000 | 4.981e+000 | 6.856e+000 |
| 8.74 | 5.002e+000 | 5.004e+000 | 4.994e+000 | 6.871e+000 |
| 8.75 | 5.015e+000 | 5.018e+000 | 5.007e+000 | 6.886e+000 |
| 8.76 | 5.028e+000 | 5.031e+000 | 5.020e+000 | 6.902e+000 |
| 8.77 | 5.041e+000 | 5.044e+000 | 5.033e+000 | 6.917e+000 |
| 8.78 | 5.054e+000 | 5.057e+000 | 5.046e+000 | 6.932e+000 |
| 8.79 | 5.067e+000 | 5.070e+000 | 5.059e+000 | 6.947e+000 |
| 8.80 | 5.081e+000 | 5.083e+000 | 5.072e+000 | 6.963e+000 |
| 8.81 | 5.094e+000 | 5.096e+000 | 5.086e+000 | 6.978e+000 |
| 8.82 | 5.107e+000 | 5.110e+000 | 5.099e+000 | 6.993e+000 |
| 8.83 | 5.120e+000 | 5.123e+000 | 5.112e+000 | 7.009e+000 |
| 8.84 | 5.133e+000 | 5.136e+000 | 5.125e+000 | 7.024e+000 |
| 8.85 | 5.147e+000 | 5.149e+000 | 5.138e+000 | 7.039e+000 |
| 8.86 | 5.160e+000 | 5.162e+000 | 5.151e+000 | 7.055e+000 |
| 8.87 | 5.173e+000 | 5.176e+000 | 5.165e+000 | 7.070e+000 |
| 8.88 | 5.186e+000 | 5.189e+000 | 5.178e+000 | 7.086e+000 |
| 8.89 | 5.200e+000 | 5.202e+000 | 5.191e+000 | 7.101e+000 |
| 8.90 | 5.213e+000 | 5.216e+000 | 5.204e+000 | 7.116e+000 |
| 8.91 | 5.226e+000 | 5.229e+000 | 5.218e+000 | 7.132e+000 |
| 8.92 | 5.240e+000 | 5.242e+000 | 5.231e+000 | 7.147e+000 |
| 8.93 | 5.253e+000 | 5.256e+000 | 5.244e+000 | 7.163e+000 |
| 8.94 | 5.267e+000 | 5.269e+000 | 5.258e+000 | 7.178e+000 |
| 8.95 | 5.280e+000 | 5.282e+000 | 5.271e+000 | 7.194e+000 |
| 8.96 | 5.293e+000 | 5.296e+000 | 5.284e+000 | 7.209e+000 |
| 8.97 | 5.307e+000 | 5.309e+000 | 5.298e+000 | 7.225e+000 |
| 8.98 | 5.320e+000 | 5.323e+000 | 5.311e+000 | 7.240e+000 |
| 8.99 | 5.334e+000 | 5.336e+000 | 5.324e+000 | 7.256e+000 |
| 9.00 | 5.347e+000 | 5.350e+000 | 5.338e+000 | 7.272e+000 |
| 9.01 | 5.361e+000 | 5.363e+000 | 5.351e+000 | 7.287e+000 |
| 9.02 | 5.374e+000 | 5.377e+000 | 5.365e+000 | 7.303e+000 |
| 9.03 | 5.388e+000 | 5.390e+000 | 5.378e+000 | 7.318e+000 |
| 9.04 | 5.401e+000 | 5.404e+000 | 5.392e+000 | 7.334e+000 |
| 9.05 | 5.415e+000 | 5.417e+000 | 5.405e+000 | 7.350e+000 |
| 9.06 | 5.428e+000 | 5.431e+000 | 5.419e+000 | 7.366e+000 |
| 9.07 | 5.442e+000 | 5.444e+000 | 5.432e+000 | 7.381e+000 |
| 9.08 | 5.455e+000 | 5.458e+000 | 5.446e+000 | 7.397e+000 |
| 9.09 | 5.469e+000 | 5.472e+000 | 5.459e+000 | 7.413e+000 |
| 9.10 | 5.483e+000 | 5.485e+000 | 5.473e+000 | 7.428e+000 |
| 9.11 | 5.496e+000 | 5.499e+000 | 5.486e+000 | 7.444e+000 |
| 9.12 | 5.510e+000 | 5.513e+000 | 5.500e+000 | 7.460e+000 |
| 9.13 | 5.524e+000 | 5.526e+000 | 5.514e+000 | 7.476e+000 |
| 9.14 | 5.537e+000 | 5.540e+000 | 5.527e+000 | 7.492e+000 |
| 9.15 | 5.551e+000 | 5.554e+000 | 5.541e+000 | 7.507e+000 |
| 9.16 | 5.565e+000 | 5.567e+000 | 5.555e+000 | 7.523e+000 |
| 9.17 | 5.579e+000 | 5.581e+000 | 5.568e+000 | 7.539e+000 |
| 9.18 | 5.592e+000 | 5.595e+000 | 5.582e+000 | 7.555e+000 |
| 9.19 | 5.606e+000 | 5.609e+000 | 5.596e+000 | 7.571e+000 |
| 9.20 | 5.620e+000 | 5.622e+000 | 5.609e+000 | 7.587e+000 |
| 9.21 | 5.634e+000 | 5.636e+000 | 5.623e+000 | 7.603e+000 |
| 9.22 | 5.648e+000 | 5.650e+000 | 5.637e+000 | 7.619e+000 |
| 9.23 | 5.661e+000 | 5.664e+000 | 5.651e+000 | 7.635e+000 |
| 9.24 | 5.675e+000 | 5.678e+000 | 5.664e+000 | 7.651e+000 |
| 9.25 | 5.689e+000 | 5.692e+000 | 5.678e+000 | 7.666e+000 |
| 9.26 | 5.703e+000 | 5.706e+000 | 5.692e+000 | 7.682e+000 |
| 9.27 | 5.717e+000 | 5.719e+000 | 5.706e+000 | 7.698e+000 |
| 9.28 | 5.731e+000 | 5.733e+000 | 5.720e+000 | 7.715e+000 |
| 9.29 | 5.745e+000 | 5.747e+000 | 5.734e+000 | 7.731e+000 |
| 9.30 | 5.759e+000 | 5.761e+000 | 5.748e+000 | 7.747e+000 |
| 9.31 | 5.773e+000 | 5.775e+000 | 5.761e+000 | 7.763e+000 |
| 9.32 | 5.787e+000 | 5.789e+000 | 5.775e+000 | 7.779e+000 |
| 9.33 | 5.801e+000 | 5.803e+000 | 5.789e+000 | 7.795e+000 |
| 9.34 | 5.815e+000 | 5.817e+000 | 5.803e+000 | 7.811e+000 |
| 9.35 | 5.829e+000 | 5.831e+000 | 5.817e+000 | 7.827e+000 |
| 9.36 | 5.843e+000 | 5.845e+000 | 5.831e+000 | 7.843e+000 |
| 9.37 | 5.857e+000 | 5.859e+000 | 5.845e+000 | 7.859e+000 |

| | | | | |
|---|---|---|---|---|
| 9.38 | 5.871e+000 | 5.873e+000 | 5.859e+000 | 7.876e+000 |
| 9.39 | 5.885e+000 | 5.888e+000 | 5.873e+000 | 7.892e+000 |
| 9.40 | 5.899e+000 | 5.902e+000 | 5.887e+000 | 7.908e+000 |
| 9.41 | 5.913e+000 | 5.916e+000 | 5.901e+000 | 7.924e+000 |
| 9.42 | 5.927e+000 | 5.930e+000 | 5.915e+000 | 7.940e+000 |
| 9.43 | 5.942e+000 | 5.944e+000 | 5.929e+000 | 7.957e+000 |
| 9.44 | 5.956e+000 | 5.958e+000 | 5.944e+000 | 7.973e+000 |
| 9.45 | 5.970e+000 | 5.972e+000 | 5.958e+000 | 7.989e+000 |
| 9.46 | 5.984e+000 | 5.987e+000 | 5.972e+000 | 8.006e+000 |
| 9.47 | 5.998e+000 | 6.001e+000 | 5.986e+000 | 8.022e+000 |
| 9.48 | 6.013e+000 | 6.015e+000 | 6.000e+000 | 8.038e+000 |
| 9.49 | 6.027e+000 | 6.029e+000 | 6.014e+000 | 8.055e+000 |
| 9.50 | 6.041e+000 | 6.044e+000 | 6.028e+000 | 8.071e+000 |
| 9.51 | 6.055e+000 | 6.058e+000 | 6.043e+000 | 8.087e+000 |
| 9.52 | 6.070e+000 | 6.072e+000 | 6.057e+000 | 8.104e+000 |
| 9.53 | 6.084e+000 | 6.086e+000 | 6.071e+000 | 8.120e+000 |
| 9.54 | 6.098e+000 | 6.101e+000 | 6.085e+000 | 8.137e+000 |
| 9.55 | 6.113e+000 | 6.115e+000 | 6.100e+000 | 8.153e+000 |
| 9.56 | 6.127e+000 | 6.129e+000 | 6.114e+000 | 8.169e+000 |
| 9.57 | 6.141e+000 | 6.144e+000 | 6.128e+000 | 8.186e+000 |
| 9.58 | 6.156e+000 | 6.158e+000 | 6.143e+000 | 8.202e+000 |
| 9.59 | 6.170e+000 | 6.173e+000 | 6.157e+000 | 8.219e+000 |
| 9.60 | 6.185e+000 | 6.187e+000 | 6.171e+000 | 8.235e+000 |
| 9.61 | 6.199e+000 | 6.201e+000 | 6.186e+000 | 8.252e+000 |
| 9.62 | 6.213e+000 | 6.216e+000 | 6.200e+000 | 8.268e+000 |
| 9.63 | 6.228e+000 | 6.230e+000 | 6.214e+000 | 8.285e+000 |
| 9.64 | 6.242e+000 | 6.245e+000 | 6.229e+000 | 8.302e+000 |
| 9.65 | 6.257e+000 | 6.259e+000 | 6.243e+000 | 8.318e+000 |
| 9.66 | 6.271e+000 | 6.274e+000 | 6.258e+000 | 8.335e+000 |
| 9.67 | 6.286e+000 | 6.288e+000 | 6.272e+000 | 8.351e+000 |
| 9.68 | 6.301e+000 | 6.303e+000 | 6.287e+000 | 8.368e+000 |
| 9.69 | 6.315e+000 | 6.318e+000 | 6.301e+000 | 8.385e+000 |
| 9.70 | 6.330e+000 | 6.332e+000 | 6.316e+000 | 8.401e+000 |
| 9.71 | 6.344e+000 | 6.347e+000 | 6.330e+000 | 8.418e+000 |
| 9.72 | 6.359e+000 | 6.361e+000 | 6.345e+000 | 8.435e+000 |
| 9.73 | 6.374e+000 | 6.376e+000 | 6.359e+000 | 8.452e+000 |
| 9.74 | 6.388e+000 | 6.391e+000 | 6.374e+000 | 8.468e+000 |
| 9.75 | 6.403e+000 | 6.405e+000 | 6.388e+000 | 8.485e+000 |
| 9.76 | 6.417e+000 | 6.420e+000 | 6.403e+000 | 8.502e+000 |
| 9.77 | 6.432e+000 | 6.435e+000 | 6.418e+000 | 8.519e+000 |
| 9.78 | 6.447e+000 | 6.449e+000 | 6.432e+000 | 8.535e+000 |
| 9.79 | 6.462e+000 | 6.464e+000 | 6.447e+000 | 8.552e+000 |
| 9.80 | 6.476e+000 | 6.479e+000 | 6.461e+000 | 8.569e+000 |
| 9.81 | 6.491e+000 | 6.493e+000 | 6.476e+000 | 8.586e+000 |
| 9.82 | 6.506e+000 | 6.508e+000 | 6.491e+000 | 8.603e+000 |
| 9.83 | 6.521e+000 | 6.523e+000 | 6.506e+000 | 8.619e+000 |
| 9.84 | 6.535e+000 | 6.538e+000 | 6.520e+000 | 8.636e+000 |
| 9.85 | 6.550e+000 | 6.553e+000 | 6.535e+000 | 8.653e+000 |
| 9.86 | 6.565e+000 | 6.567e+000 | 6.550e+000 | 8.670e+000 |
| 9.87 | 6.580e+000 | 6.582e+000 | 6.565e+000 | 8.687e+000 |
| 9.88 | 6.595e+000 | 6.597e+000 | 6.579e+000 | 8.704e+000 |
| 9.89 | 6.610e+000 | 6.612e+000 | 6.594e+000 | 8.721e+000 |
| 9.90 | 6.625e+000 | 6.627e+000 | 6.609e+000 | 8.738e+000 |
| 9.91 | 6.639e+000 | 6.642e+000 | 6.624e+000 | 8.755e+000 |
| 9.92 | 6.654e+000 | 6.657e+000 | 6.639e+000 | 8.772e+000 |
| 9.93 | 6.669e+000 | 6.672e+000 | 6.653e+000 | 8.789e+000 |
| 9.94 | 6.684e+000 | 6.687e+000 | 6.668e+000 | 8.806e+000 |
| 9.95 | 6.699e+000 | 6.702e+000 | 6.683e+000 | 8.823e+000 |
| 9.96 | 6.714e+000 | 6.717e+000 | 6.698e+000 | 8.840e+000 |
| 9.97 | 6.729e+000 | 6.732e+000 | 6.713e+000 | 8.857e+000 |
| 9.98 | 6.744e+000 | 6.747e+000 | 6.728e+000 | 8.874e+000 |
| 9.99 | 6.759e+000 | 6.762e+000 | 6.743e+000 | 8.891e+000 |
| 10.00 | 6.774e+000 | 6.777e+000 | 6.758e+000 | 8.908e+000 |

* Electronic address: `ankowski@vt.edu`

[1] P. Vogel and J. F. Beacom, Phys. Rev. D **60**, 053003 (1999).
[2] A. Strumia and F. Vissani, Phys. Lett. B **564**, 42 (2003).
[3] C. H. Llewellyn Smith, Phys. Rep. **3**, 261 (1972).
